# Supplementary material for: Cap4Video: What Can Auxiliary Captions Do for Text-Video Retrieval?
Source: arXiv:2301.00184 source file (2023-03-28)
Supplement: Supplementary file 1 [file appendix.tex]

\appendix
\section*{Appendix}
\setcounter{table}{0}
\input{supplementary/main_content}
