# Supplementary material for: Cap4Video: What Can Auxiliary Captions Do for Text-Video Retrieval?
Source: arXiv:2301.00184 source file (2023-03-28)
Supplement: Supplementary file 2 [file python_support.tex]

% Default fixed font does not support bold face
\DeclareFixedFont{\ttb}{T1}{txtt}{bx}{n}{6} % for bold
\DeclareFixedFont{\ttm}{T1}{txtt}{m}{n}{6}  % for normal

% Custom colors
\definecolor{codegreen}{rgb}{0,0.6,0}
\definecolor{codegray}{rgb}{0.5,0.5,0.5}
\definecolor{codepurple}{rgb}{0.58,0,0.82}
\definecolor{backcolour}{rgb}{0.95,0.95,0.92}

\lstdefinestyle{mystyle}{
    % backgroundcolor=\color{backcolour},   
    commentstyle=\color{codegreen},
    keywordstyle=\color{magenta},
    numberstyle=\tiny\color{codegray},
    stringstyle=\color{codepurple},
    basicstyle=\ttfamily\footnotesize,
    breakatwhitespace=false,         
    breaklines=true,                 
    captionpos=b,                    
    keepspaces=true,                 
    numbers=left,                    
    numbersep=5pt,                  
    showspaces=false,                
    showstringspaces=false,
    showtabs=false,                  
    tabsize=2
}

\lstset{style=mystyle}
